# Supplementary material for: Toward the Cure of Privacy Policy Reading Phobia: Automated Generation of Privacy Nutrition Labels From Privacy Policies
Source: arXiv:2306.10923 source file (2023-06-19)
Supplement: Supplementary file 1 [file 10_Supplementary.tex]

\section*{Appendix}
\shidong{The supplementary is in a new latex file, please check it in:}

\shidong{https://www.overleaf.com/7255942882hmbtzfjnbhmf}
